# Supplementary material for: Environment Design for Inverse Reinforcement Learning
Source: arXiv:2210.14972 source file (2024-05-14)
Supplement: Supplementary file 1 [file plot_seed_1.tex]

\begin{figure}[t]

\centering
        
         \centering
         \begin{tikzpicture}
            \draw (0, 0) node[inner sep=0] {
            \includegraphics[width=0.14\textwidth]{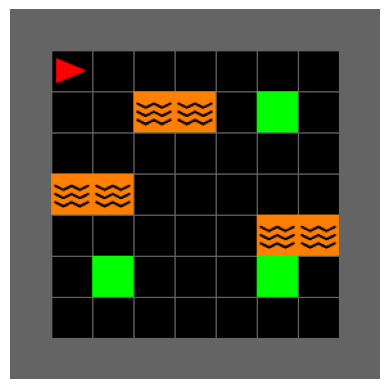}};
            \draw (0, 1.3) node {\tiny Sampled mazes (DR)};
            \draw (-1.3, 0) node {\tiny 1};
        \end{tikzpicture}
        \begin{tikzpicture}
            \draw (0, 0) node[inner sep=0] {
            \includegraphics[width=0.14\textwidth]{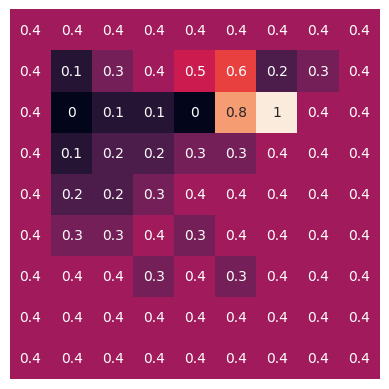}};
            \draw (0, 1.3) node {\tiny DR-BIRL};
        \end{tikzpicture}
        \begin{tikzpicture}
            \draw (0, 0) node[inner sep=0] {
            \includegraphics[width=0.14\textwidth]{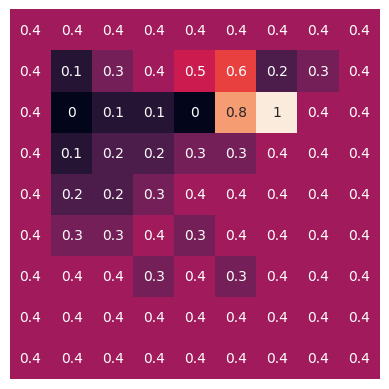}};
            \draw (0, 1.3) node {\tiny Coordinate-wise avg};
        \end{tikzpicture}
        \begin{tikzpicture}
            \draw (0, 0) node[inner sep=0] {
            \includegraphics[width=0.14\textwidth]{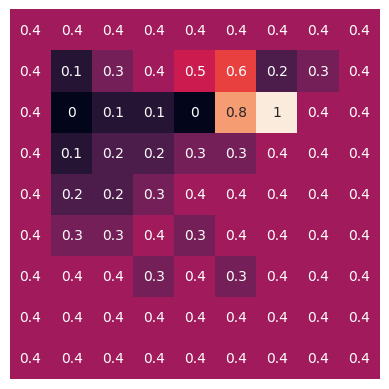}};
            \draw (0, 1.3) node {\tiny Coordinate-wise max};
        \end{tikzpicture}
        \\
         \begin{tikzpicture}
            \draw (0, 0) node[inner sep=0] {\includegraphics[width=0.14\textwidth]{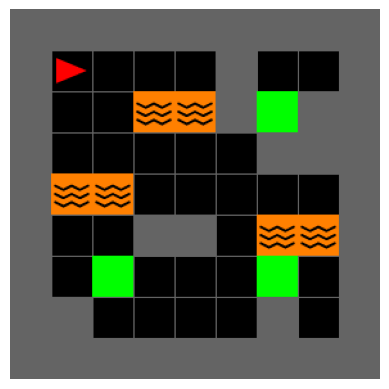}};
            \draw (-1.3, 0) node {\tiny 2};
         \end{tikzpicture}
          \includegraphics[height=0.14\textwidth]{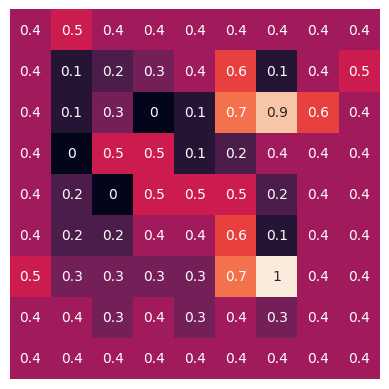} 
           \includegraphics[height=0.14\textwidth]{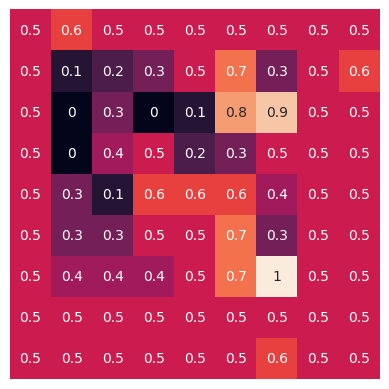} 
            \includegraphics[height=0.14\textwidth]{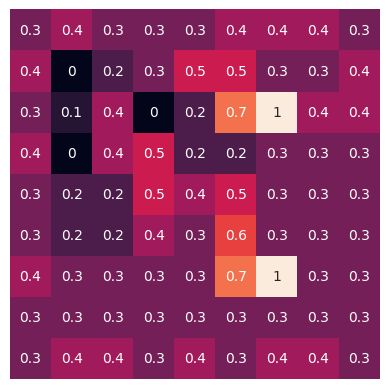} 
        \\
         \begin{tikzpicture}
            \draw (0, 0) node[inner sep=0] {\includegraphics[width=0.14\textwidth]{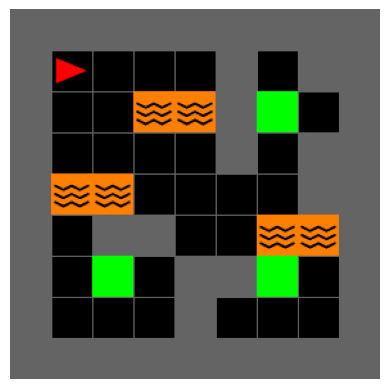}};
            \draw (-1.3, 0) node {\tiny 3};
         \end{tikzpicture}
         \includegraphics[height=0.14\textwidth]{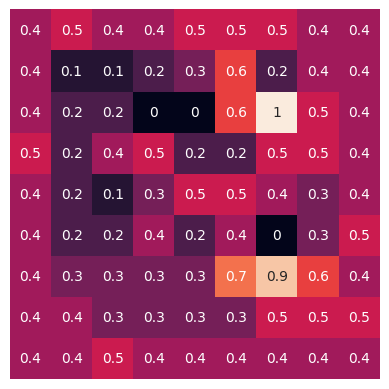} 
           \includegraphics[height=0.14\textwidth]{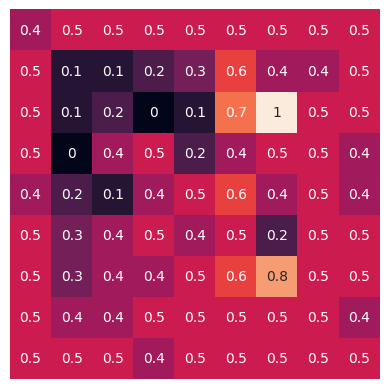} 
            \includegraphics[height=0.14\textwidth]{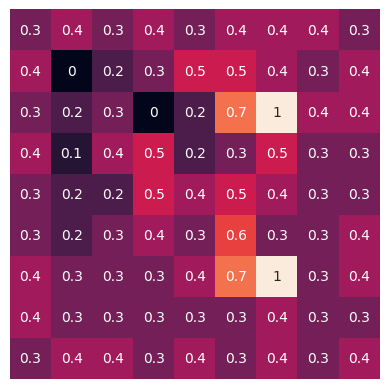}
        \\
         \begin{tikzpicture}
            \draw (0, 0) node[inner sep=0] {\includegraphics[width=0.14\textwidth]{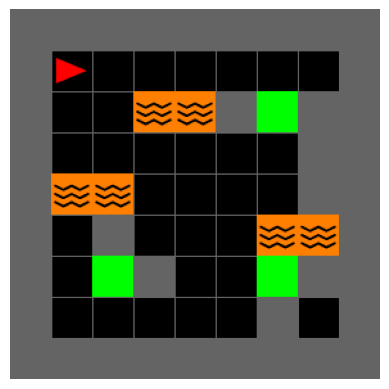}};
            \draw (-1.3, 0) node {\tiny 4};
         \end{tikzpicture}
         \includegraphics[height=0.14\textwidth]{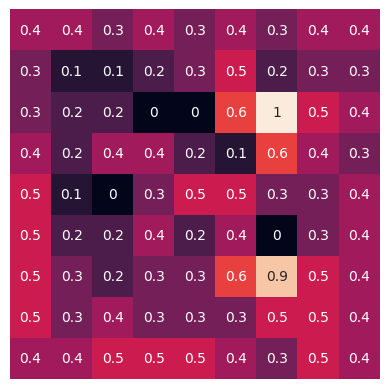} 
           \includegraphics[height=0.14\textwidth]{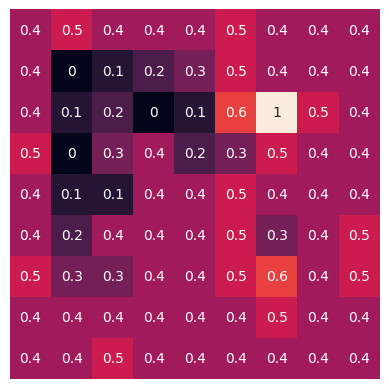} 
            \includegraphics[height=0.14\textwidth]{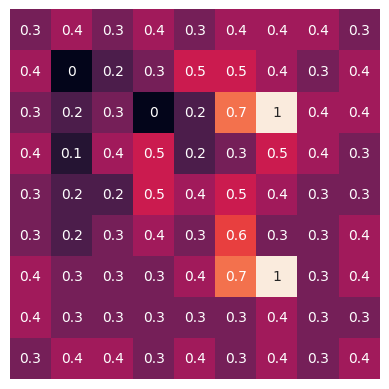} 
        \\
         \begin{tikzpicture}
            \draw (0, 0) node[inner sep=0] {\includegraphics[width=0.14\textwidth]{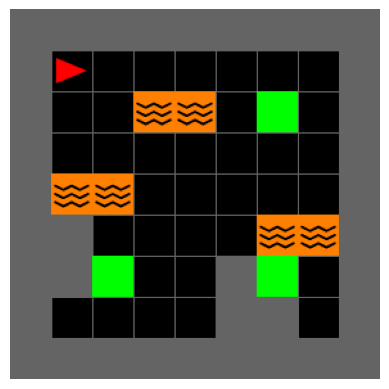}};
            \draw (-1.3, 0) node {\tiny 5};
         \end{tikzpicture}
         \includegraphics[height=0.14\textwidth]{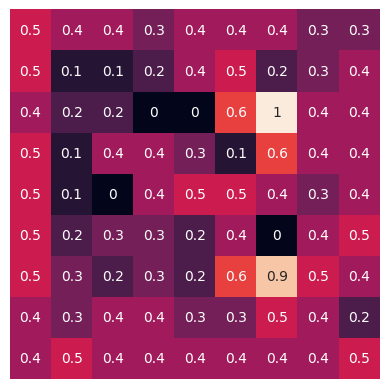} 
           \includegraphics[height=0.14\textwidth]{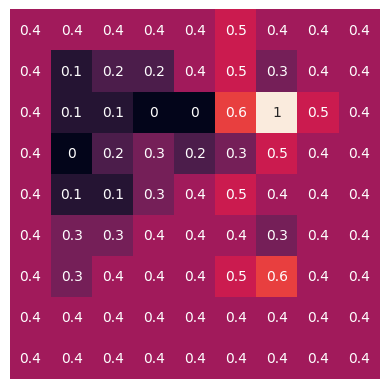} 
            \includegraphics[height=0.14\textwidth]{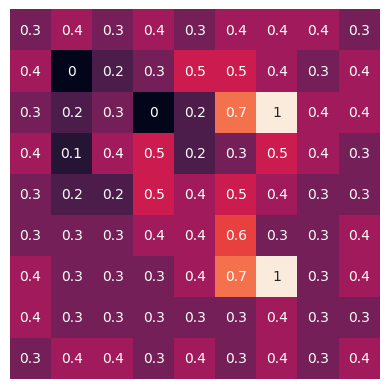}
        \\
         \begin{tikzpicture}
            \draw (0, 0) node[inner sep=0] {\includegraphics[width=0.14\textwidth]{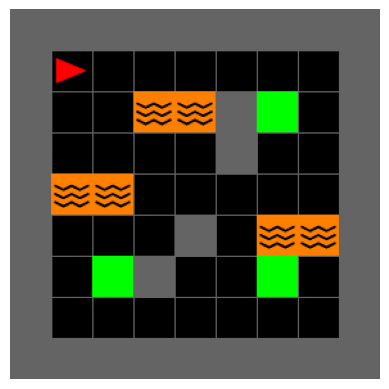}};
            \draw (-1.3, 0) node {\tiny 6};
         \end{tikzpicture}
         \includegraphics[height=0.14\textwidth]{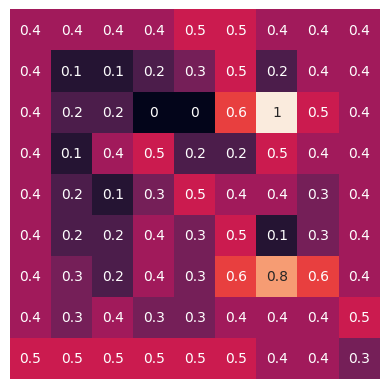} 
           \includegraphics[height=0.14\textwidth]{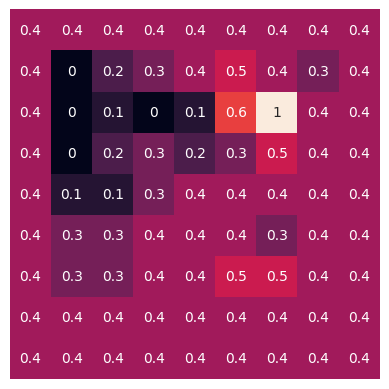} 
            \includegraphics[height=0.14\textwidth]{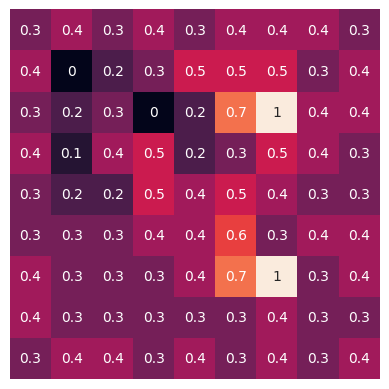} 
        \\
         \begin{tikzpicture}
            \draw (0, 0) node[inner sep=0] {\includegraphics[width=0.14\textwidth]{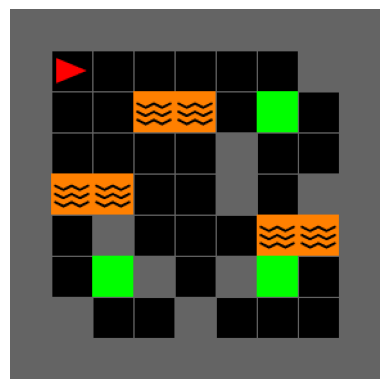}};
            \draw (-1.3, 0) node {\tiny 7};
         \end{tikzpicture}
         \includegraphics[height=0.14\textwidth]{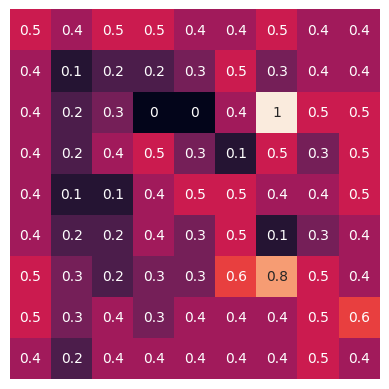} 
           \includegraphics[height=0.14\textwidth]{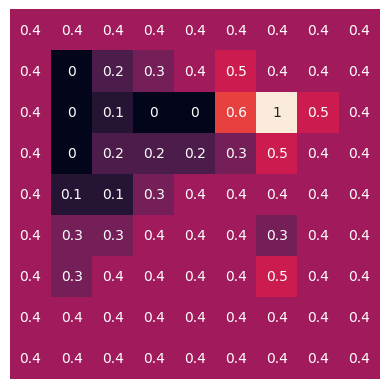} 
            \includegraphics[height=0.14\textwidth]{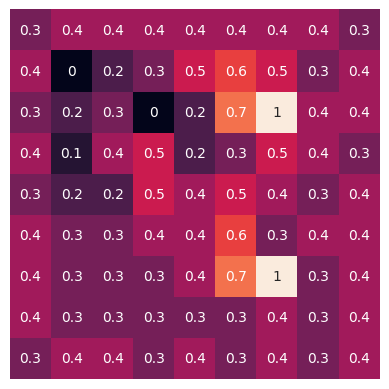} 
        \\
         \begin{tikzpicture}
            \draw (0, 0) node[inner sep=0] {\includegraphics[width=0.14\textwidth]{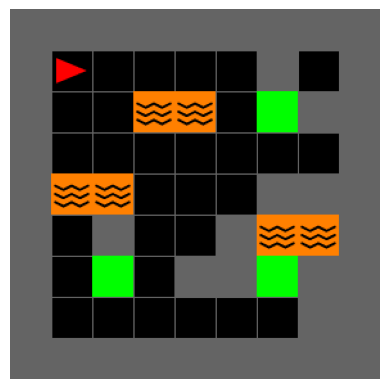}};
            \draw (-1.3, 0) node {\tiny 8};
         \end{tikzpicture}
         \includegraphics[height=0.14\textwidth]{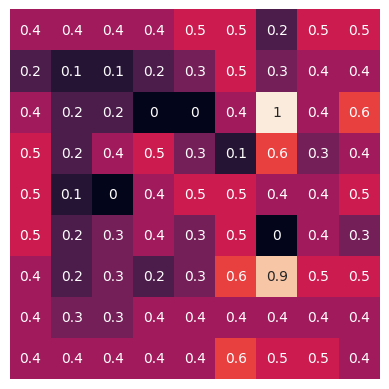} 
           \includegraphics[height=0.14\textwidth]{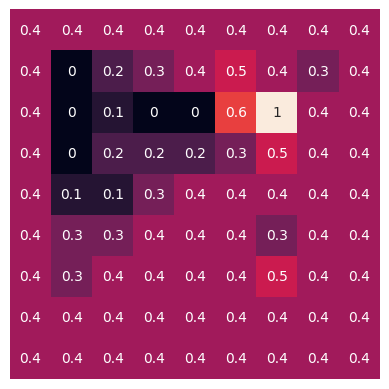} 
            \includegraphics[height=0.14\textwidth]{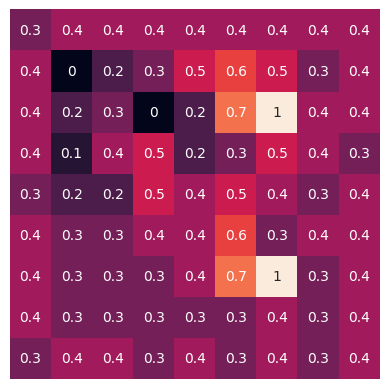}  
            
     \caption*{Run 2} 
     \label{fig:dr_additional_experiment_seed_1}
\end{figure}
